# Supplementary material for: KEVLAR-TZ: A Secure Cache for ARM TrustZone
Source: arXiv:2104.13285 source file (2021-04-27)
Supplement: Supplementary file 1 [file appendix-api.tex]

% !TEX root = ../main.tex
\section{Appendix: \sys API}\label{appendix:api}
\vs{Add some text describing this}
\begin{itemize}
{\color{red}
    \item \texttt{init\_cache(int max\_size, int hash\_size, int id\_sz, int data\_sz, int policy)}
    \item \texttt{void free\_cache(Cache *cache)}
    \item \texttt{char * cache\_query(Cache *cache, char *id)}
    \item \texttt{TEE\_Result cache\_save\_object(Cache *cache, char *id, char *data)}
}
\end{itemize}
